# Supplementary material for: Beyond Value-Function Gaps: Improved Instance-Dependent Regret Bounds for Episodic Reinforcement Learning
Source: arXiv:2107.01264 source file (2021-10-26)
Supplement: Supplementary file 1 [file thoughts.tex]

\newpage
\section{Some thoughts}

\subsection{Results for Recent Action Elimination Algorithm?}

Here are some random sketches on whether we could say anything about the action elimination algorithm by \citet{xu2021fine}.
Their algorithm uses upper- and lower-confidence bounds $\bar Q, \underline{Q}$ on $Q^\star$ in each state-action pair which are computed by a mix of (the usual) optimistic bootstrap and Monte-Carlo estimate. 
%Their Lemma~4.4 shows that the instantaneous regret in episode $k$ is bounded as
%\begin{align*}
%    \EE_{\pi_k}[V^*(S_1) - V^{\pi_k}(S_1)]
%    &\leq 2 \EE_{\pi_k}\left[ 
%    \sum_{h=1}^H
%    (\bar Q_k(S_h, A_h) - \underline Q_k(S_h, A_h)) \indicator{S_h \notin G_k}
%    \right]\\
%    &\leq 2 \EE_{\pi_k}\left[ 
%    \sum_{h=1}^H
%    \Delta Q_k(S_h, A_h)  \indicator{(S_h, A_h) \notin G_k}
%    \right]
%\end{align*}
%where $\Delta Q_k$ is what they call the range function in their Definition B.2 (an upper-bound on $\bar Q_k - \underline Q_k$ for all $(s,a)$).
%In the proof of Proposition~4.5, they show that when $s \notin G_k$, then
%\begin{align}
%    \gap(s,a) &\leq 2(\bar Q_k(s, a) - \underline Q_k(s, a)) \leq \Delta Q_k(s, a)\\
%    \gap_{\min}(s) &\leq 2(\bar Q_k(s, a) - \underline Q_k(s, a)) \leq \Delta Q_k(s, a) 
%    \label{eqn:range_gap_bound}
%\end{align}
%where $\gap_{\min}(s) = \min_{a \colon \gap(s,a) > 0} \gap(s,a)$ is the smallest non-zero gap and the second inequality holds only when there is an non-eliminated non-optimal action.
%
\begin{definition}[Range functions]
For all $s \notin G_k$ and $a \in A_k(s)$, we define
\begin{align*}
    \Delta  Q_k(s, a) &= \alpha^0_{n_k} H  
    + 4 b_{n_{k}}(s, a)
    + \sum_{t=1}^{n_{k}} \alpha^t_{n_k} \Delta  V_{k[t]}(x'_{k[t]})\\
    \Delta \ddot Q_k(s, a) &= \alpha^0_{n_k} H  
    + \clip\left[4 b_{n_{k}}(s, a) \mid \epsilon_k(s,a)\right]
    + \sum_{t=1}^{n_{k}} \alpha^t_{n_k} \Delta \ddot V_{k[t]}(x'_{k[t]})\\
    \Delta V_k(s) &= \Delta  Q_k(s, a_k) 
    \qquad \qquad \Delta \ddot V_k(s) = \Delta \ddot Q_k(s, a_k) 
\end{align*}
where $a_k = \argmax_{a \in A_k(s)} \bar Q_k(s, a) - \underline Q_k(s,a)$.
\end{definition}
Their Lemma~B.3 shows that the difference of lower and upper-bounds are bounded by this range function:
\begin{align*}
    \Delta  Q_k(s, a) &\geq \bar Q_k(s, a) - \underline Q_k(s, a)\\   
    \Delta  V_k(s) &\geq \bar V_k(s) - \underline V_k(s)
\end{align*}
for all $s,a$ (there seems to be some ambiguity here on what these range function should be for states in $G_k$.
The proof of Lemma~B.6 gives
\begin{align*}
    \EE_k[V^*(S_1) - V^{\pi_k}(S_1)]
    = \EE_k\left[ \sum_{h=B}^H \gap(S_h, A_h)\right]
    \leq 2\EE_{\pi_k}\left[ \sum_{h=B}^H \Delta Q_k(S_h, A_h)\indicator{S_h \notin G_k}\right]~.
\end{align*}
In order to get a similar result for the half-clipped range function, we need to show the following for our chosen clipping thresholds
\begin{align}
    \sum_{k=1}^T \EE_{\pi_k}\left[\sum_{h=B}^H \indicator{S_h \notin G_k}
    (\Delta  Q_k(S_h, A_h) - \Delta \ddot Q_k(S_h, A_h))\right] \leq
   \sum_{k=1}^T \EE_{\pi_k}\left[ \sum_{h=1}^H \gap(S_h, A_h)\right]
\end{align}
\begin{align*}
    \Delta  Q_k(s, a) - \Delta \ddot Q_k(s, a)
    \leq \epsilon_k(s,a) + \sum_{t=1}^{n_{k}} \alpha^t_{n_k} (\Delta V_{k}(x'_{k[t]}) - \Delta \ddot V_{k}(x'_{k[t]}))
\end{align*}

\tm{More attempts}
Lemma 4.4 in \cite{xu2021fine} seems to imply
\begin{align*}
    \EE_{k}[V^*(S_1) - V_k(S_1)|\Ecal_{k-1}] \leq 2\EE_{k}\left[\sum_{h=B}^H (\bar Q_k(S_h,A_h) - \underline Q_k(S_h,A_h))\chi(S_h\not\in G_k)\vert \Ecal_{k-1}\right],
\end{align*}
where $\Ecal_{k-1}$ is some nice event which \cite{xu2021fine} define. Our \pref{lem:clipping_gaps_rel} together with \pref{lem:gap_decomp_pi} imply that
\begin{align*}
    \frac{1}{2}\EE_{k}[V^*(S_1) - V_k(S_1)|\Ecal_{k-1}] \geq \EE_k\left[\sum_{h=B}^H \epsilon_k(S_h,A_h)\right]
\end{align*}

We can now bound the half-clipped range function from below as \cd{this doesn't work}
\begin{align*}
    &\EE_{\pi_k} \left[\sum_{h=1}^H \Delta \ddot Q_k(S_h, A_h) \indicator{S_h \notin G_k}\right]\\
    & \geq 
    \EE_{\pi_k} \left[\sum_{h=B}^H \Delta \ddot Q_k(S_h, A_h) \indicator{S_h \notin G_k}\right]\\
        & \geq 
    \EE_{\pi_k} \left[\sum_{h=B}^H (\Delta Q_k(S_h, A_h) - H \epsilon_k(S_h, A_h))\indicator{S_h \notin G_k}\right]\\
            & = 
    \EE_{\pi_k} \left[\sum_{h=B}^H \Delta Q_k(S_h, A_h)\indicator{S_h \notin G_k} \right]
    - H  \EE_{\pi_k} \left[\sum_{h=B}^H \epsilon_k(S_h, A_h))\right],
\end{align*}
where the first inequality is true because $\Delta \ddot Q_k(S_h, A_h) \indicator{S_h \notin G_k} \geq 0$ for any $h \in [H]$. The second inequality follows from
The additional $H$ factor in the second term is likely gonna hurt us but maybe this is a start. Using \eqref{eqn:range_gap_bound}, we can lower-bound the first term as
\begin{align*}
    \EE_{\pi_k}[V^*(S_1) - V^{\pi_k}(S_1)]
    = \EE_{\pi_k}\left[ \sum_{h=B}^H \gap(S_h, A_h)\right]
    \leq 2\EE_{\pi_k}\left[ \sum_{h=B}^H \Delta Q_k(S_h, A_h)\indicator{S_h \notin G_k}\right]~.
\end{align*}
Combining them gives
\begin{align*}
    &2\EE_{\pi_k} \left[\sum_{h=1}^H \Delta \ddot Q_k(S_h, A_h) \indicator{S_h \notin G_k}\right]
    \geq \EE_{\pi_k} \left[\sum_{h=B}^H (\gap(S_h, A_h) - 2H \epsilon_k(S_h, A_h))\right]~.
\end{align*}
Using the self-normalizing trick we get for any thresholds that satisfy
$  \EE_{\pi_k} \left[\sum_{h=B}^H \epsilon_k(S_h, A_h))\right]
\leq \frac{1}{4H}\EE_{\pi_k} \left[\sum_{h=B}^H \gap(S_h, A_h) \right]$
\begin{align*}
    \EE_{\pi_k}[V^*(S_1) - V^{\pi_k}(S_1)]
    &=\EE_{\pi_k} \left[\sum_{h=B}^H \gap(S_h, A_h) \right] - \frac{1}{2}\EE_{\pi_k} \left[\sum_{h=B}^H \gap(S_h, A_h) \right]
    \\
    &\leq \EE_{\pi_k} \left[\sum_{h=B}^H \gap(S_h, A_h) \right] - 2H \EE_{\pi_k} \left[\sum_{h=B}^H \epsilon_k(S_h, A_h) \right]
    \\
    & \leq
    2\EE_{\pi_k} \left[\sum_{h=1}^H \Delta \ddot Q_k(S_h, A_h) \indicator{S_h \notin G_k}\right]
\end{align*}
\subsection{Correctness things to be double-checked}
\begin{enumerate}
\item Corollary 8 needs to be stated differently or proved differently. We do pay a gap in state-action pairs that can be visited by some suboptimal policy even if there is an optimal policy passing through it.
See also the discussion around $\widetilde \gap$ vs. $\returngap$ below.
\item Figure out $V^* \leq 1$ vs $V^*  < 1$ issue in general lower-bound
\item Avoid uniqueness assumptions and notation of optimal policies in the upper-bounds
Double-check the bounds stated in the table in Figure 1
\item Clean up and ensure consistency in Appendix C.3 (“value function” vs. “return”)
Double-check the simplified optimization lemma in the main text matches the one in the appendix.
\end{enumerate}
\subsection{Suggestions}
\paragraph{Why policy-dependent gap?} What is the benefit for using a policy-dependent gap? We argue that this helps in Figure 1 but the improved clipping is also sufficient to give the desired rate in Figure 1 (and in the example in D.2). I currently do not know any concrete example where optimizing over $\pi^*_k$ is beneficial. If there is one, we should include it in the paper and otherwise remove this optimization.
\paragraph{State full-support lower bound more generally} State the full-support bound in the more general way and have the condition in the sum -- similar to what we have in the table in Figure 1?

\paragraph{Some generalization / equivalent to notion of return gap in stochastic MDPs?}

Let $B = \min\{ h \in [H+1] \colon \gap(S_h, A_h) > 0 \}$ be the first time a non-zero gap is encountered. Note that $B$ is a stopping time w.r.t. the filtration $\mathcal{F}_h = \sigma(S_1, A_1, \dots, S_h, A_h)$. Further let
\begin{align}
    \Bcal(s,a) \equiv \{B \leq \kappa(s), S_{\kappa(s)} = s, A_{\kappa(s)} = a\} 
\end{align}
be the event that $(s,a)$ was visited after a non-zero gap in the episode.
We now define this notion of average gap:
\begin{align}
    \widetilde{\gap}_k(s,a) \equiv 
    \begin{cases}
    \frac{1}{H}
    \EE_{\pi_k}\left[ \sum_{h=1}^H \gap(S_h, A_h) ~ \bigg| ~\Bcal(s,a) \right]
    & \textrm{if }\PP_{\pi_k}(\Bcal(s,a)) > 0\\
    \infty & \textrm{otherwise}
    \end{cases}
\end{align}
The condition for the first case ensures that the conditional expectation is unique.
For any suboptimal state-action pair $(s,a)$ (i.e. that satisfies $\gap(s,a) >0$), the expression in the first case simplifies to just $\frac{1}{H}
    \EE_{\pi_k}\left[ \sum_{h=1}^H \gap(S_h, A_h) ~ \bigg| ~S_{\kappa(s)} = s, A_{\kappa(s)} = a \right]$, the average gap conditioned on the policy visiting $(s,a)$.

Using this definition, we can state our main result as
\begin{theorem}[Informal]
The regret $\regret(K)$ of \texttt{StrongEuler} is bounded as
\begin{align*}
    \regret(K) \lessapprox&~
    \sum_{s,a} \min_{k \in [K]} \left\{
    \frac{\Vcal^*(s,a)}{\gap(s,a) + \widetilde{\gap}_k(s,a)}
    + \sqrt{\Vcal^*(s,a) (K - k)}\right\} \log(K)
        \\&
     + \sum_{s,a} SH^3 \log\frac{MK}{\delta} \min\left\{ \log \frac{MK}{\delta}, \log \frac{MH}{\gap(s,a) + \widetilde \gap(s,a)}\right\}
     \\& + SAH^3 (S \vee H)\log\frac{M}{\delta}.
    %O\Bigg(\log(K)\max_{\pi_{1:K}}\min_{\pi^*_{1:K}}\sum_{(s,a) \in \Scal\times\Acal} \min_{t\in %[K]}\Bigg\{\frac{\Vcal_{\max_t}(s,a)}{\breve \gap_{\pi_t}^{\pi^*_t}(s,a)} + %\sum_{k=t+1}^K\frac{\Vcal_{\max_k}(s,a)}{\sum_{j=t+1}^k \breve %\gap_{\pi_j}^{\pi^*_j}(s,a)}\Bigg\}\Bigg).
\end{align*}
\end{theorem}

We can also remove the dependency on the random policy $\pi_k$ by taking the minimum over all policies in the gap definition as
\begin{align}
    \widetilde{\gap}(s,a) \equiv \min_{\substack{\pi \in \Pi \colon \\\PP_{\pi}(\Bcal(s,a)) > 0}}&~
    \frac{1}{H}
    \EE_{\pi}\left[ \sum_{h=1}^H \gap(S_h, A_h) ~ \bigg| ~\Bcal(s,a) \right]\\
     = \min_{\substack{\pi \in \Pi \colon \\\PP_{\pi}(\Bcal(s,a)) > 0}}&~
    \frac{1}{H}
    \EE_{\pi}\left[ \sum_{h=1}^{\kappa(s)} \gap(S_h, A_h) ~ \bigg| ~\Bcal(s,a) \right]
\end{align}
Then the main regret upper-bound becomes
\begin{align*}
    \regret(K) \lessapprox&~
    \sum_{s,a} 
    \frac{\Vcal^*(s,a)}{\gap(s,a) + \widetilde{\gap}(s,a)} \log(K)
        \\&
     + \sum_{s,a} SH^3 \log\frac{MK}{\delta} \min\left\{ \log \frac{MK}{\delta}, \log \frac{MH}{\gap(s,a) + \widetilde \gap(s,a)}\right\}
     \\& + SAH^3 (S \vee H)\log\frac{M}{\delta}.
    %O\Bigg(\log(K)\max_{\pi_{1:K}}\min_{\pi^*_{1:K}}\sum_{(s,a) \in \Scal\times\Acal} \min_{t\in %[K]}\Bigg\{\frac{\Vcal_{\max_t}(s,a)}{\breve \gap_{\pi_t}^{\pi^*_t}(s,a)} + %\sum_{k=t+1}^K\frac{\Vcal_{\max_k}(s,a)}{\sum_{j=t+1}^k \breve %\gap_{\pi_j}^{\pi^*_j}(s,a)}\Bigg\}\Bigg).
\end{align*}
Comparison to other notions of gap:
To see how much we might have lost when removing the policy-dependency, we compare this gap to other notions:
\begin{align}
\widetilde \gap(s,a) & > 0\\
    \widetilde \gap(s,a) &\geq \frac{\gap(s,a)}{H}\\
    \widetilde \gap(s,a) &\geq \frac{\gap_{\min}}{H}\\
    \widetilde \gap(s,a) & = \frac{\returngap(s,a)}{H} \quad \textrm{when } \returngap(s,a) > 0\\
    \widetilde \gap(s,a) & \geq \frac{\returngap(s,a)}{H} 
\end{align}

\paragraph{Tightness of upper-bound in MDPs with deterministic transitions}
There is a discrepancy between $\widetilde \gap(s,a)$ and $\returngap(s,a)$ because $\widetilde \gap(s,a)$ takes the minimum over all policies that visit $(s,a)$ and have made a mistake before but $\returngap(s,a)$ only takes the minimum over all policies that visit $(s,a)$. When $(s,a)$ can be visited through an optimal and a suboptimal policy, then  $\returngap(s,a) = 0$ but $0 < \widetilde \gap(s,a) < \infty$. Those pairs thus appear in the upper-bound but not in the regret lower-bound. Note that this is not an issue of writing things as $\widetilde \gap$ but also occurs in our results as currently written. 

Essentially there are 3 cases in MDPs with deterministic transitions:
\begin{itemize}
    \item The state-action pair can only be visited by a suboptimal policy: We are tight with the lower-bound up to a $H^2$ factor. \cmark
    \item The state-action pair cannot be visited by any suboptimal policy: Neither our lower-bound nor our upper bound pays for such pairs. \cmark
    \item The state-action pair can be visited by an optimal and a suboptimal policy: These pairs do not appear in the lower-bound but we pay for them with average gap across the episode in the upper-bound.
    \xmark
\end{itemize}
I think we might be able to tighten our upper-bound regret analysis to show that we can also clip state-action pairs of the 3rd case to $\infty$ in deterministic MDPs.

A key property we need to prove and use for this is
\begin{align}
    \EE_{\pi_k}\left[ \sum_{h=B}^{h'} E_k(S_h, A_h) \right] \geq 
\EE_{\pi_k}\left[ \sum_{h=B}^{h'} \gap(S_h, A_h) \right] \end{align}
for all $h' \in [H]$ (or maybe only as long as $\pi_k$ is optimal from $h'$ on?). Recall the surplus definition $E_k(s,a) = \bar Q_k(s,a) - r(s,a) - \langle P(\cdot | s,a) , \bar V_k \rangle$ and the form $\bar Q_k$ which is
\begin{align*}
\bar Q_k(s,a) = H \wedge \widehat r(s,a) + \langle \widehat P(\cdot | s,a), \bar V_k \rangle + \textrm{bonus}(s,a)    
\end{align*}
The usual notion of optimism gives this inequality for $h' = H$.

\paragraph{Deriving the key property for deterministic MDPs:} Let the bonus added at episode $k$ for state-action pair $(s,a)$ be $b_k(s,a)$. 
For a deterministic policy $\pi$, denote the (deterministic) trajectory of state-action pairs be $s_1^\pi, a_1^\pi, \dots, s_H^\pi, a_H^\pi$.
We assume that there is a layer $h'$ such that there is a $\hat \pi \in \Pi$ with $V^{\hat \pi} = V^*$ and  $(s_h^{\hat \pi}, a_h^{\hat \pi}) = (s_h^{\pi_k}, a_h^{\pi_k})$ for all $h \geq h'$.
%Let $h'$ be a layer of the MDP at which there exists a $\pi^* \in \Pi^*$ such that $\pi_k(s) = \pi^*(s)$ where $\kappa(s) = h'$ \cd{Should this be $h' \geq \kappa(s)$?}. 
Because we are considering deterministic transitions we can write 
\begin{align*}
    \EE_{\pi_k}\left[\sum_{h=B}^{h'} \gap(S_h,A_h)\right] &= \sum_{h=B}^{h'} \gap(s_h^{\pi_k},a_h^{\pi_k})\\
    \EE_{\pi_k}\left[ \sum_{h=B}^{h'} E_k(S_h, A_h) \right] &= \sum_{h=B}^{h'} E_k(s_h^{\pi_k}, a_h^{\pi_k})
\end{align*} where where $s_h^{\pi}$ denotes the state visited by $\pi$ at time $h$. Note that $B$ is also fixed given $\pi_k$ in deterministic MDPs. 
Euler computes the optimistic Q-function as $\bar Q_k(s,a) = H \wedge \hat r_k(s,a) + \langle \hat P_k(\cdot|s,a), \bar V_k \rangle + b_k(s,a)$.
There are two cases which we treat separately:
\paragraph{Case 1: $(s,a)$ has been visited often enough so that $\bar Q_k(s,a) = \hat r_k(s,a) + \langle \hat P_k(\cdot|s,a), \bar V_k \rangle + b_k(s,a)$:} 
Since the MDP is deterministic, we have $\hat P_k(\cdot|s,a) = P(\cdot|s,a)$. This implies that $E_k(s,a) = \hat r_k(s,a) - r(s,a) + b_k(s,a)$. Further, we can write the sum of the gaps as 
\begin{align*}
    \sum_{h=1}^{h'} \gap(s^{\pi_k}_h,a^{\pi_k}_h) &= V^{*}(s^{\pi_k}_1) - V^{\pi_k}(s^{\pi_k}_1) - \left(V^{*}(s^{\pi_k}_{h'+1}) - V^{\pi_k}(s^{\pi_k}_{h'+1})\right)\\
    &= V^{*}(s^{\pi_k}_1) - V^{\pi_k}(s^{\pi_k}_1)\\
    &= \sum_{h=B}^{H} (r(s_h^{\hat \pi},a_h^{\hat \pi}) - r(s_h^{\pi_k},a_h^{\pi_k}))
    = \sum_{h=B}^{h'} (r(s_h^{\hat \pi},a_h^{\hat \pi}) - r(s_h^{\pi_k},a_h^{\pi_k})).
\end{align*}
Because we have picked $\pi_k$ at episode $k$ it further must hold that $\bar V^{\pi_k}(s_1) \geq \bar V^{\hat \pi}(s_1)$ but what is more it must hold that $\sum_{h=1}^{h'} \hat r(s_h^{\pi_k},a_h^{\pi_k}) + b_{k}(s_h^{\pi_k},a_h^{\pi_k}) \geq \sum_{h=1}^{h'} \hat r(s_h^{\hat \pi},a_h^{\hat \pi}) + b_{k}(s_h^{\hat \pi},a_h^{\hat \pi})$ as otherwise the policy which follows $\hat \pi$ up to $h'$ and $\pi_k$ from $h'+1$ to $H$ would have higher value function in the empirical MDP \cd{this assumes that all sa along the paths of both policies have been visited often enough so that the optimistic Q-function does not get clipped}. Further, because the bonuses include optimism of the rewards it holds that $\sum_{h=1}^{h'} \hat r(s_h^{\hat \pi},a_h^{\hat \pi}) + b_{k}(s_h^{\hat \pi},a_h^{\hat \pi}) \geq \sum_{h=1}^{h'} r(s_h^{\hat \pi},a_h^{\hat \pi})$ with high probability. This implies
\begin{align*}
    \sum_{h=1}^{h'}\gap(s_h^{\pi_k},a_h^{\pi_k}) &= \sum_{h=1}^{h'} r(s_h^{\hat \pi},a_h^{\hat \pi}) - r(s_h^{\pi_k},a_h^{\pi_k}) \leq \sum_{h=1}^{h'} \hat r(s_h^{\pi_k},a_h^{\pi_k}) - r(s_h^{\pi_k},a_h^{\pi_k}) +  b_{k}(s_h^{\pi_k},a_h^{\pi_k})\\
    &=\sum_{h=1}^{h'} E_k(s_h^{\pi_k},a_h^{\pi_k}).
\end{align*}
\paragraph{Case 2: $(s,a)$ has not been visited often enough so that $\bar Q_k(s,a) = H < \hat r(s,a) + \langle \hat P(\cdot|s,a), \bar V_k \rangle + b_k(s,a)$:} 
\cd{We need to handle this case as well. Clipping to $H$ is somewhat non-optional in Euler and ideally we can handle clipping here directly. If this turns out to be difficult, we may bound the number of episodes where a clipped optimistic Q-function could occur. This could be made easier by clipping to 2H instead (which should also be sufficient) and bound the number of times until $b_k(s,a) \leq H$.}

\paragraph{Both cases at the same time?} Let $\bar \pi_k$ be the policy which follows $\hat\pi$ up to and including layer $h'$, and from $h'+1$ to $H$ it follows $\pi_k$. Then we know that it must hold $\bar V^{\bar\pi}(s_{h'+1}) \geq \bar V^{\hat\pi}(s_{h'+1})$ as otherwise the policy which follows $\pi_k$ until $h'$ and then follows $\hat\pi$ would have higher value function than $\pi_k$. Suppose we can show that $\sum_{h=1}^{h'} r(s_h^{\hat \pi},a_h^{\hat \pi}) \leq \bar V^{\bar \pi}(s_1) - \bar V^{\bar\pi}(s_{h'+1}^{\pi_k})$. Then we could write
\begin{align*}
    \sum_{h=1}^{h'} r(s_h^{\hat \pi},a_h^{\hat \pi}) - r(s_h^{\pi_k},a_h^{\pi_k}) 
    & \leq 
    \bar V^{\bar \pi}(s_1) - \bar V^{\bar \pi}(s_{h'+1}^{\pi_k}) - \sum_{h=1}^{h'} r(s_h^{\pi_k},a_h^{\pi_k})\\
    &= \bar V^{\bar \pi}(s_1) - \bar V_k(s_{h'+1}^{\pi_k}) - \sum_{h=1}^{h'} r(s_h^{\pi_k},a_h^{\pi_k})\\
    &\leq \bar V_k(s_1) - \bar V_k(s_{h'+1}^{\pi_k}) - \sum_{h=1}^{h'} r(s_h^{\pi_k},a_h^{\pi_k}).
\end{align*}
Further, it holds
\begin{align*}
    \sum_{h=1}^{h'} E_k(s_h^{\pi_k},a_h^{\pi_k}) &= \sum_{h=1}^{h'} \bar V_k(s_h^{\pi_k}) - r(s_h^{\pi_k},a_h^{\pi_k}) - \langle P(\cdot|s_h^{\pi_k},a_h^{\pi_k}), \bar V_k \rangle\\
    &=\sum_{h=1}^{h'} \bar V_k(s_h^{\pi_k}) - \sum_{h=2}^{h'+1} \bar V_k(s_h^{\pi_k}) - \sum_{h=1}^{h'} r(s_h^{\pi_k},a_h^{\pi_k})\\
    &= \bar V_k(s_1) - \bar V_k(s_{h'+1}^{\pi_k})- \sum_{h=1}^{h'} r(s_h^{\pi_k},a_h^{\pi_k}).
\end{align*}
Combining with the inequality on the sum of rewards we arrive at the desired result. To show $\sum_{h=1}^{h'} r(s_h^{\hat \pi},a_h^{\hat \pi}) \leq \bar V^{\bar \pi}(s_1) - \bar V^{\bar\pi}(s_{h'+1}^{\pi_k})$ argue as follows. Let $\tilde h$ be the smallest layer for which $\bar V^{\bar \pi}(s_{\tilde h}^{\hat\pi}) = H - \tilde h + 1$. Because $\bar V^{\bar\pi}(s_{h'+1}^{\pi_k}) \leq H-h'$ we have
\begin{align*}
    \bar V^{\bar \pi}(s_1) - \bar V^{\bar\pi}(s_{h'+1}^{\pi_k}) &= \bar V^{\bar \pi}(s_1) - \bar V^{\bar \pi}(s_{\tilde h}^{\hat\pi}) + \bar V^{\bar \pi}(s_{\tilde h}^{\hat\pi}) - \bar V^{\bar \pi}(s_{h'+1}^{\hat\pi})\\
    &\geq \bar V^{\bar \pi}(s_1) - \bar V^{\bar \pi}(s_{\tilde h}^{\hat\pi}) + h' - \tilde h + 1 \geq \bar V^{\bar \pi}(s_1) - \bar V^{\bar \pi}(s_{\tilde h}^{\hat\pi}) + \sum_{h=\tilde h}^{h'} r(s_h^{\hat\pi},a_h^{\hat\pi}).
\end{align*}
Finally by our definition of $\tilde h$ it must hold that for all $h < \tilde h$, $\hat r(s_h^{\hat\pi},a_h^{\hat\pi}) + b_k(s_h^{\hat\pi},a_h^{\hat\pi}) \leq 1$ and hence we can write $\bar V^{\bar\pi}(s_1) = \sum_{h=1}^{\tilde h-1} \hat r(s_h^{\hat\pi},a_h^{\hat\pi}) + b_k(s_h^{\hat\pi},a_h^{\hat\pi}) + \bar V^{\bar \pi}(s_{\tilde h}^{\hat\pi})$, which implies
\begin{align*}
    \bar V^{\bar \pi}(s_1) - \bar V^{\bar \pi}(s_{\tilde h}^{\hat\pi}) \geq \sum_{h=1}^{\tilde h-1} \hat r(s_h^{\hat\pi},a_h^{\hat\pi}) + b_k(s_h^{\hat\pi},a_h^{\hat\pi}) \geq \sum_{h=1}^{\tilde h-1} r(s_h^{\hat\pi},a_h^{\hat\pi}),
\end{align*}
where the last inequality holds with probability $1-\delta$ because $\hat r(s_h^{\hat\pi},a_h^{\hat\pi}) + b_k(s_h^{\hat\pi},a_h^{\hat\pi}) \geq r(s_h^{\hat\pi},a_h^{\hat\pi})$ for all $h \in [H], (s,a) \in \Scal\times\Acal$ by the construction of the bonuses.

It would be interesting if could show something similar for non-deterministic transitions. In particular if there exists a layer $h'$ such that with probability $1$ $\pi_k$ agrees with $\Pi^*$ on every state in the layer then does the inequality between surpluses and gaps still hold up to $h'$?

\paragraph{The argument for non-deterministic transitions:} Assume that at time $h'$ it holds that there exists an optimal policy $\hat \pi$ (not necessarily deterministic), such that $\pi_k$ and $\hat\pi$ have the same distribution over state-action pairs $(s,a)$ at $h'$. Define $\bar\pi$ as in the deterministic transitions MDP case, i.e., $\bar\pi$ matches $\pi_k$ from layer $h'+1$ to $H$ and otherwise follows $\hat\pi$ from layer $1$ to layer $h'$. Suppose we can show $\EE_{\hat\pi}[\sum_{h=1}^{h'}r(S_h,A_h)] \leq \bar V^{\bar\pi}(s_1) - \EE_{\pi_k}[\bar V_k(S_{h'+1})]$. We can write
\begin{align*}
    \EE_{\hat\pi}\left[\sum_{h=1}^{h'} r(S_h,A_h)\right] \leq V^{\bar\pi}(s_1) - \EE_{\pi_k}[\bar V_k(S_{h'+1})] \leq \bar V_k(s_1) - \EE_{\pi_k}[\bar V_k(S_{h'+1})].
\end{align*}
Further we have
\begin{align*}
    \EE_{\pi_k}\left[\sum_{h=1}^{h'} E_k(S_h,A_h)\right] &= \EE_{\pi_k}\left[\sum_{h=1}^{h'} \bar V_k(S_h) - r(S_h,A_h) - \langle P(\cdot|S_h,A_h), \bar V_k \rangle\right]\\
    &= \EE_{\pi_k}\left[\sum_{h=1}^{h'} \bar V_k(S_h) - \EE_{\pi_k}\left[\bar V_k(S_{h+1})|S_h\right]\right] - \sum_{h=1}^{h'}\EE_{\pi_k}[r(S_h,A_h)]\\
    &=\bar V_k(s_1) - \EE_{\pi_k}[\bar V_k(S_{h'+1})] - \sum_{h=1}^{h'}\EE_{\pi_k}[r(S_h,A_h)].
\end{align*}
Next we decompose the sum of the gaps as a difference of rewards by using Lemma~\ref{lem:gap_decomp_pi}
\begin{align*}
\EE_{\pi_k}\left[\sum_{h=1}^{h'} \gap(S_h,A_h)\right] &= \EE_{\pi_k}\left[\sum_{h=1}^{H} \gap(S_h,A_h)\right] - \EE_{\pi_k}\left[\sum_{h=h'+1}^{H} \gap(S_h,A_h)\right]\\
&= V^{\hat\pi}(s_1) - V_k(s_1) - \EE_{\pi_k}\left[\EE_{\pi_k}\left[\sum_{h=h'+1}^{H} \gap(S_h,A_h)|S_{h'+1}=s_{h'+1}\right]\right]\\
&= \EE_{\hat\pi}\left[\sum_{h=1}^H r(S_h,A_h)\right] - \EE_{\pi_k}\left[\sum_{h=1}^H r(S_h,A_h)\right]\\
&- \EE_{\pi_k}\left[\EE_{\pi_k}\left[V^{\hat\pi}(s_{h'+1})|S_{h'+1}=s_{h'+1}\right] -\EE_{\pi_k}\left[ V_k(s_{h'+1})|S_{h'+1}=s_{h'+1}\right]\right]\\
&\overset{(i)}{=} \EE_{\hat\pi}\left[\sum_{h=1}^H r(S_h,A_h)\right] - \EE_{\pi_k}\left[\sum_{h=1}^H r(S_h,A_h)\right]\\
&-\EE_{\hat\pi}\left[V^{\hat\pi}(S_{h'+1})\right] + \EE_{\pi_k}\left[V_k(S_{h'+1})\right]\\
&=\EE_{\hat\pi}\left[\sum_{h=1}^H r(S_h,A_h)\right] - \EE_{\pi_k}\left[\sum_{h=1}^H r(S_h,A_h)\right]\\
&-\EE_{\hat\pi}[\sum_{h=h'+1}^H r(S_h,A_h)] + \EE_{\pi_k}[\sum_{h=h'+1}^H r(S_h,A_h)]\\
&= \EE_{\hat\pi}\left[\sum_{h=1}^{h'} r(S_h,A_h)\right] - \EE_{\pi_k}\left[\sum_{h=1}^{h'}r(S_h,A_h)\right],
\end{align*}
where $(i)$ follows from the fact that $\pi_k$ and $\hat\pi$ have the same distribution over state-action pairs in layer $h'$ and hence $\PP_{\hat\pi}(S_{h'+1} = s_{h'+1}) = \PP_{\pi_k}(S_{h'+1} = s_{h'+1})$.
Combining the above with the inequality on difference of rewards and the equality for surpluses we have
\begin{align*}
    \EE_{\pi_k}\left[\sum_{h=1}^{h'} \gap(S_h,A_h)\right] &= \EE_{\hat\pi}\left[\sum_{h=1}^{h'} r(S_h,A_h)\right] - \EE_{\pi_k}\left[\sum_{h=1}^{h'}r(S_h,A_h)\right]\\
    &\leq \bar V_k(s_1) - \EE_{\pi_k}[\bar V_k(S_{h'+1})] - \sum_{h=1}^{h'}\EE_{\pi_k}[r(S_h,A_h)]\\
    &=\EE_{\pi_k}\left[\sum_{h=1}^{h'} E_k(S_h,A_h)\right].
\end{align*}

Next we try to show $\EE_{\hat\pi}[\sum_{h=1}^{h'}r(S_h,A_h)] \leq \bar V^{\bar\pi}(s_1) - \EE_{\pi_k}[\bar V_k(S_{h'+1})]$ or equivalently $\EE_{\bar\pi}[\sum_{h=1}^{h'}r(S_h,A_h)] + \EE_{\bar\pi}[\bar V^{\bar\pi}(S_{h'+1})]\leq \bar V^{\bar\pi}(s_1)$. Fix $(s_h,a_h) \in \bar\pi$ and consider 
\begin{align*}
    r(s_h,a_h) + \mathbb{E}_{\bar\pi}[\bar V^{\bar\pi}(S_{h+1}) ~|~ S_h = a_h, A_h = a_h] = r(s_h,a_h) + \langle P(\cdot|s_h,a_h),\bar V^{\bar\pi} \rangle.
\end{align*}
It either holds that $\bar V^{\bar\pi}(s_h) = H-h+1$ or $\bar V^{\bar\pi}(s_h) = \hat r(s_h,a_h) + b_k^{rw}(s_h,a_h) + b_k^{prob}(s_h,a_h)+ b_k^{str}(s_h,a_h) + \langle \hat P(\cdot|s_h,a_h), \bar V^{\bar\pi} \rangle$.
Suppose that $\bar V^{\bar\pi}(s_h) = H-h+1$, then we must have $r(s_h,a_h) \leq 1 \leq \bar V^{\bar\pi}(s_h) - \langle P(\cdot|s_h,a_h),\bar V^{\bar\pi} \rangle$. Otherwise we have
\begin{align*}
    r(s_h,a_h) &\leq \hat r(s_h,a_h) + b_k^{rw}(s_h,a_h) = \bar V^{\bar\pi}(s_h) - b_k^{prob}(s_h,a_h) - b_k^{str}(s_h,a_h) - \langle \hat P(\cdot|s_h,a_h), \bar V^{\bar\pi} \rangle\\
    &=\bar V^{\bar\pi}(s_h) - \langle P(\cdot|s_h,a_h), \bar V^{\bar\pi} \rangle\\
    &+ \langle P(\cdot|s_h,a_h) - \hat P(\cdot|s_h,a_h), \bar V^{\bar\pi} \rangle - b_k^{prob}(s_h,a_h) - b_k^{str}(s_h,a_h).
\end{align*}
By definition of $\bar V^{\bar\pi}$ it holds that $\bar V^{\hat\pi}(s_h) \leq \bar V^{\bar\pi}(s_h) \leq \bar V_k(s_h)$ on all $s_h$, because $\pi_k$ is the Bellman optimal policy with respect to the empirical MDP. This implies we can use Lemma F.2 in \citep{simchowitz2019non} to show that $|\langle P(\cdot|s_h,a_h) - \hat P(\cdot|s_h,a_h), \bar V^{\bar\pi} \rangle| \leq b_k^{prob}(s_h,a_h)$ and thus $r(s_h,a_h) \leq \bar V^{\bar\pi}(s_h) - \langle P(\cdot|s_h,a_h), \bar V^{\bar\pi} \rangle$. Combining everything, we have
\begin{align*}
    \EE_{\bar\pi}\left[\sum_{h=1}^{h'}r(S_h,A_h)\right] + \EE_{\bar\pi}[\bar V^{\bar\pi}(S_{h'+1})]&= \EE_{\bar\pi}\left[\sum_{h=1}^{h'-1}r(S_h,A_h)\right] + \EE_{\bar\pi}[r(S_{h'},A_{h'})+ \langle P(\cdot|S_{h'},A_{h'}),\bar V^{\bar\pi}\rangle]\\
    &\leq \EE_{\bar\pi}\left[\sum_{h=1}^{h'-1}r(S_h,A_h)\right] + \EE_{\bar\pi}[\bar V^{\bar\pi}(S_{h'})] \leq \ldots \leq \bar V^{\bar\pi}(s_1).
\end{align*}

\subsection{Extension to linear MDPs?}

I do not think the clipped surplus bound we derive relies on finite state-spaces. We could also think about what a good definition of clipping threshold $\epsilon_k$ would be in linear MDPs \citep{jin2020provably}.
From a quick look, I think Lemma~B.4 by \citet{jin2020provably} ensures that the surpluses of their LSVI-UCB algorithm satisfy
\begin{align}
    0 \leq E_k(s,a) \leq 2 \beta \sqrt{\phi(s,a)^\top \Lambda_k^{-1} \phi(s,a)}. 
\end{align}
This means their algorithm is strongly optimistic and our surplus clipping bound from \pref{prop:surplus_clipping_bound} gives
\begin{align}
    &V^\star(s_1) - V^{\pi_k}(s_1)\\
    &\leq 4 \EE_{\pi_k} \left[ \sum_{h=1}^H \clip \left[ E_k(S_h,A_h) ~ \bigg| ~ \frac{1}{4}\gap(S_h,A_h) \vee \epsilon_k(S_h,A_h) \right] \right]\\
    & \leq 
    4\EE_{\pi_k} \left[ \sum_{h=1}^H \clip \left[ 2 \beta \sqrt{\phi(S_h,A_h)^\top \Lambda_k^{-1} \phi(S_h,A_h)} ~ \bigg| ~ \frac{1}{4}\gap(S_h,A_h) \vee \epsilon_k(S_h,A_h) \right] \right].
\end{align}
Assume for now, we settle for $\epsilon(s,a) = \inf_k (\gap(s,a) \vee \epsilon_k(s,a) )$, a policy independent clipping threshold. Then we have to bound an expression of the form
\begin{align*}
    \regret(T)
    \lesssim \sum_{h=1}^H \sum_{k=1}^T \EE_{\pi_k} \left[ \clip\left[\sqrt{\phi(S_h,A_h)^\top \Lambda_k^{-1} \phi(S_h,A_h)} ~ \bigg| ~ \epsilon(S_h,A_h) \right] \right]
\end{align*}
where $\Lambda_k$ is the regularized covariance matrix with all features up to episode $k-1$.
Handling this expression is not trivial but having a good gap-dependent bound for linear MDPs would certainly be a nice contribution.

\paragraph{Idea how to proceed:}
One could possibly get a $\gap_{\min}$ bound by noticing that 
\begin{align*}
    \EE_{\pi_k} \left[ \clip\left[\sqrt{\phi(S_h,A_h)^\top \Lambda_k^{-1} \phi(S_h,A_h)} ~ \bigg| ~ \epsilon(S_h,A_h) \right] \right] &\leq \EE_{\pi_k} \left[\frac{\phi(S_h,A_h)^\top \Lambda_k^{-1} \phi(S_h,A_h)}{\epsilon(S_h,A_h)} \right]\\
    &\leq \EE_{\pi_k} \left[\frac{\phi(S_h,A_h)^\top \Lambda_k^{-1} \phi(S_h,A_h)}{\gap_{\min}} \right],
\end{align*}
and then argue similarly to how the log-det lemmas are proved for the contextual linear bandits problems. 

Taking this idea a little further -- instead of replacing all $\epsilon(S_h,A_h)$ by $\gap_{\min}$ we can partition the gaps into $O(\log(T))$ ranges as follows. Define a grid on the interval $[1,T]$ (could also be $[1,\sqrt{T}]$) such that there are $O(\log(T))$ partitions. The first partition includes all gaps in $[1/2,1]$, the second all gaps in $[1/4,1/2]$, etc., where the last partition includes gaps in $[2/T, T]$. Now we can replace $\epsilon(S_h,A_h)$ by the lower limit of the partition in which it falls e.g., if $\epsilon(S_h,A_h) \in [1/2^{\ell}, 1/2^{\ell+1}]$, then bound
\begin{align*}
    \clip\left[\sqrt{\phi(S_h,A_h)^\top \Lambda_k^{-1} \phi(S_h,A_h)} ~ \bigg| ~ \epsilon(S_h,A_h) \right] \leq
    \frac{\phi(S_h,A_h)^\top \Lambda_k^{-1} \phi(S_h,A_h)}{1/2^{\ell+1}}.
\end{align*}
Now, we could try to come up with a better version of the log-det lemma which uses the fact that $\epsilon(S_h,A_h) > 1/2^{\ell+1}$ to shave off factors of dimensionality from the sum over terms grouped in the $\ell$-th interval.

\paragraph{The formal argument:} We first note that \pref{lem:Vdd_lb1} only requires that the algorithm be optimistic i.e. $\bar Q_k(s,a) \geq Q^*(s,a), \forall (s,a) \in \Scal\times\Acal$. Lemma B.5 in \cite{jin2020provably} guarantees that optimism holds for their algorithm $\textsc{LSVI-UCB}$, where the Q-functions are defined as $\hat Q_k(s,a) := \min(\langle \phi(s,a), \mathbf{w}^{k}_{\kappa(s)} \rangle + \beta\sqrt{\phi(s,a)^\top (\Lambda^k)_{\kappa(s)}^{-1}\phi(s,a)} H)$, where $\mathbf{w}^k_{\kappa(s)}$ are the weights computed by the algorithm at episode $k$ for layer $\kappa(s)$ and $\Lambda^k_{\kappa(s)}$ is the design matrix at episode $k$ for layer $\kappa(s)$. We can now apply \pref{prop:surplus_clipping_bound} with $\epsilon_k(s,a) = \gap_{\min}/H$ to bound the regret at episode $k$ as
\begin{align*}
    V^*(s_1) - V^{\pi_k}(s_1) \leq 4\EE_{\pi_k}\left[\sum_{h=B}^H\clip[E_k(S_h,A_h)|\epsilon_k(S_h,A_h)]\right].
\end{align*}
Further we have that
\begin{align*}
    E_k(s,a) = \hat Q_k(s,a) - r(s,a) - \langle P(\cdot|s,a),\hat V_k \rangle  &\leq  \langle \phi(s,a), \mathbf{w}^k_{\kappa(s)} \rangle + \beta\sqrt{\phi(s,a)^\top (\Lambda^k_{\kappa(s)})^{-1}\phi(s,a)}\\
    &- r(s,a) - \langle P(\cdot|s,a),\hat V_k\rangle\\
    &= \langle \phi(s,a), \mathbf{w}^k_{\kappa(s)} \rangle - Q^*(s,a) - \langle P(\cdot|s,a),\hat V_k - V^*\rangle\\
    &+\beta\sqrt{\phi(s,a)^\top (\Lambda^k_{\kappa(s)})^{-1}\phi(s,a)}\\
    &\leq 2\beta\sqrt{\phi(s,a)^\top (\Lambda^k_{\kappa(s)})^{-1}\phi(s,a)},
\end{align*}
where the last inequality follows from Lemma B.4 in \citet{jin2020provably}. And so we can bound the regret as
\begin{align*}
    \regret(T) &\leq 4\sum_{k=1}^K\sum_{h=1}^H \EE_{\pi_k}\left[\clip\left[2\beta\sqrt{\phi(S_h,A_h)^\top (\Lambda^k_h)^{-1}\phi(S_h,A_h)} \vert \epsilon_k(S,A)\right]\right]\\
    &\leq 4\sum_{k=1}^K\sum_{h=1}^H \EE_{\pi_k}\left[\frac{4\beta^2\phi(S_h,A_h)^\top (\Lambda^k_{h})^{-1}\phi(S_h,A_h)}{\epsilon_k(S_h,A_h)}\right]\\
    &\leq16H\beta^2\sum_{h=1}^H\sum_{k=1}^K \EE_{\pi_k}\left[\frac{\phi(S_h,A_h)^\top (\Lambda^k_{h})^{-1}\phi(S_h,A_h)}{\gap_{\min}}\right]\\
    &\leq \frac{32H^2\beta^2d\log(2dT/\delta)}{\gap_{\min}} = O\left(\frac{d^3H^4\log^2(dT/\delta)}{\gap_{\min}}\right),
\end{align*}
where the last inequality follows from Lemma D.2 in \citet{jin2020provably}, in the following way. Since $\Lambda_h^k$ is a random variable depending on $\pi_{1:k-1}$ we can further take the expectation for a fixed $h$ as
\begin{align*}
    \sum_{k=1}^K \EE_{\pi_{1:k}}[\phi(S_h,A_h)^\top (\Lambda^k_{h})^{-1}\phi(S_h,A_h)] = \EE_{\pi_{1:K}}\left[\sum_{k=1}^K\phi(S_h,A_h)^\top (\Lambda^k_{h})^{-1}\phi(S_h,A_h)\right],
\end{align*}
and now apply Lemma D.2 in \citet{jin2020provably} for every realization of state-action pairs at layer $h$ played throughout the $K$ episodes.

\section{Tighter Clipping for Optimal Pairs Reachable Similarly by an Optimal Policy}

\begin{lemma}\label{lem:Oclipping_perfect}
Let $\Ocal \subseteq [H]$ be the set of time steps where for every $h \in \Ocal$ there is an optimal policy $\pi^\star$ such that $\PP_{\pi^\star}(S_h, A_h) = \PP_{\pi_k}(S_h, A_h)$. Then
\begin{align}
    \EE_{\pi_k} \left[\sum_{h=1}^H \gap(S_h, A_h)\right] \leq 
    \EE_{\pi_k} \left[ \sum_{h = 1}^{H} \indicator{h \notin \Ocal} E_k(S_h, A_h)\right].
\end{align}
\end{lemma}
\cd{I think this may be too strong to be true? I will first show a weaker version:}
\begin{lemma}Assume strong optimism and greedy $\bar V_k$, i.e., $\bar V_k(s) \geq \max_{a} \bar Q_k(s,a)$ for all $s \in \Scal$.
Let $\Ocal \subseteq [H]$ be the set of time steps such that there is an optimal policy $\pi^\star$ which satisfies $\PP_{\pi^\star}(S_h, A_h) = \PP_{\pi_k}(S_h, A_h)$ for every $h \in \Ocal$. Then
\begin{align}
    \EE_{\pi_k} \left[\sum_{h=1}^H \gap(S_h, A_h)\right] \leq 
    \EE_{\pi_k} \left[ \sum_{h = 1}^{H} \indicator{h \notin \Ocal} E_k(S_h, A_h)\right].
\end{align}
\end{lemma}
\begin{proof}
We show this by proving that for any $\underline{h}, \bar h \in \Ocal$ with $\underline{h} \leq \bar h$, we have
\begin{align*}
    \EE_{\pi_k} \left[\sum_{h=\underline h + 1}^{\bar h - 1} \gap(S_h, A_h)\right] \leq 
    \EE_{\pi_k} \left[ \sum_{h=\underline h + 1}^{\bar h - 1}  E_k(S_h, A_h)\right].
\end{align*}
Since $\gap(S_h ,A_h) = 0$ for $h \in \Ocal$ and we can assume that there is a dummy $H+1 \in \Ocal$, this is sufficient to prove the statement to show.
We now rewrite both sides of the inequality as
\begin{align*}
    \EE_{\pi_k} \left[ \sum_{h=\underline h + 1}^{\bar h - 1}  E_k(S_h, A_h)\right]
    &=
     \EE_{\pi_k} \left[
     \bar V_k(S_{\underline h + 1}) - \bar V_k(S_{\bar h})
     + \sum_{h=\underline h + 1}^{\bar h - 1} r(S_h, A_h)
     \right]\\
     \EE_{\pi_k} \left[\sum_{h=\underline h + 1}^{\bar h - 1} \gap(S_h, A_H)\right]
     &=
     \EE_{\pi_k} \left[ V^\star(S_{\underline h + 1}) - V^{\pi_k}(S_{\underline h + 1}) - 
     V^\star(S_{\bar h}) + V^{\pi_k}(S_{\bar h})
     \right]\\
     &=\EE_{\pi_k} \left[ V^\star(S_{\underline h + 1}) - 
     V^\star(S_{\bar h}) + \sum_{h=\underline h + 1}^{\bar h - 1} r(S_h, A_h)
     \right].
\end{align*}
\textcolor{olive}{JZ: isn't there a sign error in front of the rewards in the first line? If I am correct this breaks the whole proof.}
Thus, it suffices to show
$\EE_{\pi_k} \left[ V^\star(S_{\underline h + 1}) - 
     V^\star(S_{\bar h}) \right] \leq 
     \EE_{\pi_k} \left[
     \bar V_k(S_{\underline h + 1}) - \bar V_k(S_{\bar h})\right]$.
     Note that since $P_{\pi_k}(S_{\underline h}, A_{\underline h}) = P_{\pi^\star}(S_{\underline h}, A_{\underline h})$, this also implies that 
     $P_{\pi_k}(S_{\underline h + 1}) = P_{\pi^\star}(S_{\underline h + 1})$ by the Markov property of the MDP. Hence
\begin{align*}
    \EE_{\pi_k} \left[ V^\star(S_{\underline h + 1}) - 
     V^\star(S_{\bar h}) \right]
     = 
     \EE_{\pi^\star} \left[ V^\star(S_{\underline h + 1}) - 
     V^\star(S_{\bar h}) \right]
     = \EE_{\pi^\star} \left[
     \sum_{h=\underline h + 1}^{\bar h - 1} r(S_h, A_h)
     \right]
\end{align*}
and all that is left to show is
\begin{align*}
    \EE_{\pi^\star}\left[ 
    \bar V_k(S_{\underline h + 1})
    \right] \geq 
    \EE_{\pi^\star}\left[ 
    \sum_{h=\underline h + 1}^{\bar h - 1} r(S_h, A_h)
    +
    \bar V_k(S_{\bar h })
    \right].
\end{align*}
This holds due to strong optimism and the greedy nature of $\bar V_k$ by \pref{lem:multi_strong_optimism}.
\end{proof}

\begin{lemma}[Multi-step Strong Optimism]
\label{lem:multi_strong_optimism}
Assume an algorithm is strongly optimistic and it computes its optimistic V-function greedily based on its optimistic Q-function, i.e.,  $\bar V_k(s) \geq \bar Q_{k}(s,a)$ holds always. Then it satisfies in all rounds $k$, stopping times $N, N'$ with $N \leq N'$ a.s. and policies $\pi$ that
\begin{align*}
    \EE_{\pi}\left[ 
    \bar V_k(S_{N})
    -
    \sum_{t=N}^{N' - 1} r(S_t, A_t)
    +
    \bar V_k(S_{N'})
    \right] \geq 0.
\end{align*}
\end{lemma}
This property can be seen as a multi-step generalization of strong optimism. While strong optimism only considers the surplus in one time-step, we here consider the surplus over multiple time steps under any policy.
\cd{This lemma definitely holds when $N$ and $N'$ are regular indices. The stopping time version should be double-checked carefully!}
\begin{proof} We lower-bound the LHS in the condition as
\begin{align*}
  &\EE_{\pi}\left[ 
    \bar V_k(S_{N})
    -
    \sum_{t=N}^{N' - 1} r(S_t, A_t)
    +
    \bar V_k(S_{N'})\right]
    \\
    &= \EE_{\pi}\left[\indicator{N < N'}\left( 
    \bar V_k(S_{N})
    -
    \sum_{t=N}^{N' - 1} r(S_t, A_t)
    +
    \bar V_k(S_{N'})\right)\right]\\
    & \overset{(i)}{\geq} 
    \EE_{\pi}\left[ \indicator{N < N'}\left(
    \bar Q_k(S_{N}, A_N)
    -
    \sum_{t=N}^{N' - 1} r(S_t, A_t)
    +
    \bar V_k(S_{N'})\right)\right] \\
     & = 
    \EE_{\pi}\left[ \indicator{N < N'}\left(
    E_k(S_N, A_N)
    + \bar V_k(S_{N+1}) -
    \sum_{t=N+1}^{N' - 1} r(S_t, A_t)
    +
    \bar V_k(S_{N'}) \right)\right] \\
     & = 
    \EE_{\pi}\left[ \indicator{N < N'}
    E_k(S_N, A_N)\right]\\
    & \qquad + 
    \EE_{\pi}\left[ \indicator{N + 1 < N'}
    \left(\bar V_k(S_{N+1}) -
    \sum_{t=N+1}^{N' - 1} r(S_t, A_t)
    +
    \bar V_k(S_{N'}) \right)\right] \\
    & \overset{(ii)}{\geq} 
    \EE_{\pi}\left[\sum_{t=N}^{N' - 1} E_k(S_t, A_t) \right].
\end{align*}
where step $(i)$ follows from how the greedy assumption of $\bar V_k$ and step $(ii)$ is a recursive application of the previous steps. Finally, $\EE_{\pi}\left[\sum_{t=N}^{N' - 1} E_k(S_t, A_t) \right] \geq 0$ holds because of strong optimism.
\end{proof}
\textcolor{olive}{JZ: I think the proof of the Lemma above is flawed, here is an alternative which might be simpler.}
\begin{lemma}
\label{lem:gap_surp_bound_jul}
Assume strong optimism and greedy $\bar V_k$, i.e., $\bar V_k(s) \geq \max_{a} \bar Q_k(s,a)$ for all $s \in \Scal$.
Let $\Ocal \subseteq [H]$ be the set of time steps such that there is an optimal policy $\pi^\star$ which satisfies $\PP_{\pi^\star}(S_h, A_h) \geq \PP_{\pi_k}(S_h, A_h)$ for every $h \in \Ocal$. Then
\begin{align}
    \EE_{\pi_k} \left[\sum_{h=1}^H \gap(S_h, A_h)\right] \leq 
    \EE_{\pi_k} \left[ \sum_{h = 1}^{H} \indicator{h \notin \Ocal} E_k(S_h, A_h)\right].
\end{align}
\end{lemma}
\begin{proof}
Define the following value function:
\begin{align*}
    \bar V_{k,h_0}^\pi(s) &= \EE_{\pi}\left[\sum_{h=h_0}^H E_k(S_h,A_h)+r(S_h,A_h)\,\middle\vert\,S_{h_0}=s\right]\\
    &= E_k(s_0,\pi(s_0))+r(s_0,\pi(s_0)) + \langle P(\cdot|s_0,\pi(s_0)), \bar V^\pi_{k,h_0+1}\rangle\,,
\end{align*}
where 
$\bar V_{k,H+1}^\pi=0$ by convention.
First we show that for all $\pi$: $\bar V_{k}^\pi\leq \bar V_k$.
This holds trivially for $H+1$, so by induction given that $\bar V_{k,h+1}^\pi\leq \bar V_{k,h+1}$
\begin{align*}
    \bar V_{k,h}^\pi(s) &= E_k(s,\pi(s))+r(s,\pi(s)) + \langle P(\cdot|s,\pi(s)), \bar V^\pi_{k,h+1}\rangle\\
    &\leq E_k(s,\pi(s))+r(s,\pi(s)) + \langle P(\cdot|s,\pi(s)), \bar V_{k,h+1}\rangle\\
    &=\bar Q_{k,h}(s,\pi(s))\leq \bar V_{k,h}(s)\,.
\end{align*}
Having established $\bar V_{k}^\pi\leq \bar V_k$, we have
\begin{align*}
    \EE_{\pi_k} \left[\sum_{h=1}^H \gap(S_h, A_h)\right] &= V^{\pi^*}_0-V^{\pi_k}_0\\
    &\leq V^{\pi^*}_0-\bar V^{\pi^*}_{k,0}+\bar V^{\pi_k}_{k,0}-V^{\pi_k}_0\\
    &= \EE_{\pi_k} \left[ \sum_{h = 1}^{H}  E_k(S_h, A_h)\right]-\EE_{\pi^*} \left[ \sum_{h = 1}^{H}  E_k(S_h, A_h)\right]\\
    &\leq \EE_{\pi_k} \left[ \sum_{h = 1}^{H} \indicator{h \notin \Ocal} E_k(S_h, A_h)\right]\,.
\end{align*}
\end{proof}
Using this result, we can get a version of \pref{lem:Vdd_lb1} that takes $\Ocal$ into account. It holds in any MDP but is never worse than \pref{lem:Vdd_lb1} in deterministic MDPs. In stochastic MDPs this may yield a worse bound because the stopping time $B$ is missing. We may be able also add it though.

\begin{lemma}
% \label{lem:Vdd_lb1_dett}
Let $\epsilon_k : \Scal \times \Acal \rightarrow \RR^+_0$ be arbitrary and let $\Ocal \subseteq H$ be the set of time steps such that there is an optimal policy $\pi^\star$ which satisfies $\PP_{\pi^\star}(S_h, A_h) \geq \PP_{\pi_k}(S_h, A_h)$ for every $h \in \Ocal$. Then for any strongly and greedily optimistic algorithm (which satisfies  $\bar V_k$, i.e., $\bar V_k(s) \geq \max_{a} \bar Q_k(s,a)$ for all $s \in \Scal$), it holds that 
\begin{align*}
    \label{eq:clipped_ineq_tight_det}
    \ddot V_k(s_1) - V^{\pi_k}(s_1) &\geq 
    \EE_{\pi_k}\left[
    \sum_{h=1}^H \indicator{h \notin \Ocal} \left( \gap(S_{h},A_h) - \epsilon_{k}(S_{h}, A_h)\right)
    \right]\\
    &= \EE_{\pi_k}\left[
    \sum_{h=1}^H  \left( \gap(S_{h},A_h) -
    \indicator{h \notin \Ocal}\epsilon_{k}(S_{h}, A_h)\right)
    \right]
\end{align*}
\end{lemma}

\tm{We can most likely prove something stronger from Lemma~\ref{lem:gap_surp_bound_jul} which also simplifies a lot or removes a lot of the proofs. Sketch below:}
Let $\tilde \Ocal_k = \{(s,a) \in \Scal\times\Acal: \PP_{\pi_k}(S_{\kappa(s)} = s, A = a) \leq \PP_{\pi^*}(S_{\kappa(s)} = s, A = a)\}$ be the set of state-action pairs which have higher probability to visited by $\pi^*$ than $\pi_k$. By Lemma~\ref{lem:Vdd_lb1} we have
\begin{align*}
    \ddot V_k(s_1) - V^{\pi_k}(s_1) &
    \geq \EE_{\pi_k}\left[\sum_{h=B}^{H} \ddot E_k(S_h,A_h)\right]\\
    & \geq \EE_{\pi_k}\left[\sum_{h=B}^{H}
    \indicator{(S_h,A_h) \not\in \tilde\Ocal_k}
    \ddot E_k(S_h,A_h)\right]\\
    %&\geq \EE_{\pi_k}\left[\sum_{h=B}^{H} E_k(S_h,A_h)\right] - \EE_{\pi_k}\left[\sum_{h=B}^{H} \epsilon_k(S_h,A_h)\right]\\
    &\geq \EE_{\pi_k}\left[\sum_{h=B}^{H}\chi((S_h,A_h) \not\in \tilde\Ocal_k) E_k(S_h,A_h)\right] - \EE_{\pi_k}\left[\sum_{h=B}^{H}\chi((S_h,A_h) \not\in \tilde\Ocal_k) \epsilon_k(S_h,A_h)\right],
    % \ddot V_k(s_1) - V^{\pi_k}(s_1) &= \EE_{\pi_k}\left[\sum_{h=1}^{H}\ddot E_k(S_h,A_h)\right] \geq \EE_{\pi_k}\left[\sum_{h=1}^{H}\chi((S_h,A_h) \not\in \tilde\Ocal_k)\ddot E_k(S_h,A_h)\right]\\
    % &\geq \EE_{\pi_k}\left[\sum_{h=1}^{H}\chi((S_h,A_h) \not\in \tilde\Ocal_k) E_k(S_h,A_h)\right] - \EE_{\pi_k}\left[\sum_{h=1}^{H}\chi((S_h,A_h) \not\in \tilde\Ocal_k) \epsilon_k(S_h,A_h)\right].
\end{align*}
where $B$ is the stopping time for the process defined by $\pi_k$ matching $\pi^*$.
Next we use Lemma~\ref{lem:gap_surp_bound_jul} to lower bound $\EE_{\pi_k}\left[\sum_{h=B}^{H}\chi((S_h,A_h) \not\in \tilde\Ocal_k) E_k(S_h,A_h)\right]$. Recall that from the proof of the lemma it follows that
\begin{align*}
    \EE_{\pi_k}\left[\sum_{h=1}^H\gap(S_h,A_h)\right] \leq \EE_{\pi_k}\left[\sum_{h=1}^HE_k(S_h,A_h)\right] - \EE_{\pi^*}\left[\sum_{h=1}^H E_k(S_h,A_h)\right].
\end{align*}
Fix $h$ and consider the difference \begin{align*}
    \EE_{\pi_k}[E_k(S_h,A_h)] - \EE_{\pi^*}[E_k(S_h,A_h)] &= \sum_{(s,a): \kappa(s)=h} \left(\PP_{\pi_k}(S_h=s,A_h=a) - \PP_{\pi^*}(S_h=s,A_h=a)\right)E_k(s,a)\\
    &\leq \sum_{(s,a) \not\in \tilde \Ocal_k} \PP_{\pi_k}(S_h=s,A_h=a)E_k(s,a)\\
    &= \EE_{\pi_k}[\chi((S_h,A_h)\not\in \tilde\Ocal_k)E_k(S_h,A_h)].
\end{align*}
\tm{Unfortunately I don't know how to introduce the stopping time in the difference of expectations because $\Acal_h$ depends on $\pi_k$ but is independent of the randomness in $\pi^*$. Further if we do not have the stopping time then Lemma~\ref{lem:clipping_gaps_rel} will fail.}
\begin{align*}
    \ddot V_k(s_1) - V^{\pi_k}(s_1) &= \EE_{\pi_k}\left[\sum_{h=1}^{H}\ddot E_k(S_h,A_h)\right] \geq \EE_{\pi_k}\left[\sum_{h=1}^{H}\chi((S_h,A_h) \not\in \tilde\Ocal_k)\ddot E_k(S_h,A_h)\right]\\
    &\geq \EE_{\pi_k}\left[\sum_{h=1}^{H}\chi((S_h,A_h) \not\in \tilde\Ocal_k) E_k(S_h,A_h)\right] - \EE_{\pi_k}\left[\sum_{h=1}^{H}\chi((S_h,A_h) \not\in \tilde\Ocal_k) \epsilon_k(S_h,A_h)\right]\\
    &\geq \EE_{\pi_k}\left[\sum_{h=1}^{H}\chi((S_h,A_h) \not\in \tilde\Ocal_k) E_k(S_h,A_h)\right] - \EE_{\pi_k}\left[\sum_{h=B}^{H} \epsilon_k(S_h,A_h)\right],
\end{align*}
where the last inequality follows because if $\chi(\Acal_h) = 1$ this implies that $\forall h' < h$, $\chi((S_{h'},A_{h'}) \not\in \tilde O_k) = 0$ and hence
\begin{align*}
    \EE_{\pi_k}\left[\sum_{h=1}^{H}\chi((S_h,A_h) \not\in \tilde\Ocal_k) \epsilon_k(S_h,A_h)\right] \leq \EE_{\pi_k}\left[\sum_{h'=h}^{H}\chi(\Acal_{h}) \epsilon_k(S_{h'},A_{h'})\right].
\end{align*}
The above implies 
\begin{align*}
    \EE_{\pi_k}\left[\sum_{h=B}^{H} \epsilon_k(S_h,A_h)\right] = \sum_{h=1}^{H}\EE_{\pi_k}\left[\sum_{h'=h}^{H}\chi(\Acal_{h}) \epsilon_k(S_{h'},A_{h'})\right] \geq \EE_{\pi_k}\left[\sum_{h=1}^{H}\chi((S_h,A_h) \not\in \tilde\Ocal_k) \epsilon_k(S_h,A_h)\right].
\end{align*}

\cd{Fill in the proof for this which follows the proof of \pref{lem:Vdd_lb1} for the most part.}

\cd{This lemma is sufficient for us to be able to clip all states-action pairs at times in $\Ocal$ to whatever we want (e.g. $\infty$).}

\cd{Could formulate $\Ocal$ as a set of state-action pairs and have $\underline h$ and $\bar h$ just be stopping times of when a pair in $\Ocal$ is reached?}

\cd{The current result doesn't quite give us the optimal regret rate for deterministic MDPs. For this, we would need a stronger version of \pref{lem:Oclipping_perfect}} where $\Ocal$ can be covered by multiple optimal policies.

% \subsection{Putting everything together}

\subsection{Negative result for deterministic transitions?}

Consider the MDP in Figure~\ref{fig:mdp_det_lower}. This MDP has $2n+9$ states and $4n+8$ actions. The rewards for each action are either $1/12$ or $1/12+\epsilon/2$ and can be found next to the transitions from the respective states. We are going to label the states according to their layer and their position in the layer so that the first state is $s_{1,1}$ the state which is to the left of $s_{1,1}$ in layer 2 is $s_{2,1}$ and to the right $s_{2,2}$. In general the $i$-th state in layer $h$ is denoted as $s_{h,i}$. The rewards in all states but $s_{4,1},s_{4,2}$ and $s_{5,i}$ for all $i>1$ are deterministic. The rewards for $s_{4,2}$ and $s_{5,i}$ for all $i>1$ are Bernoulli with mean $1/12$ according to the figure. Further the rewards at state $s_{4,1}$ are Bernoulli with mean $1/12+\epsilon/2$ for the action leading to $s_{5,1}$ and $1/12$ for the action leading to $s_{5,2}$. From the construction it is clear that $V^*(s_{1,1}) = 1/2+\epsilon$. Further there are two sets of optimal policies with the above value function -- the $n$ optimal policies which visit state $s_{2,2}$ and the $n$ optimal policies which visit $s_{4,1}$. Notice that the information theoretic lower bound for this MDP is in $O(\log(K)/\epsilon)$ as only the state $s_{4,2}$ does not belong to an optimal policy. In particular, there is no dependence on $n$. Next we try to show that the class of optimistic algorithms will incur regret at least $\Omega(n\log(K)/\epsilon)$.
\paragraph{Class of algorithms.}
We adopt the class of algorithms from Section G.2 in \citep{simchowitz2019non} with an additional assumption which we clarify momentarily. Recall that the class of algorithms assumes access to an optimistic value function $\bar V_k(s) \geq V^*(s)$ and optimistic Q-functions. 
In particular the algorithms construct optimistic Q and value functions as
\begin{align*}
    \bar V_k(s) &= \max_{a\in\Acal} \bar Q_k(s,a)\\
    Q_k(s,a) &= \hat r_k(s,a) + b_k^{rw}(s,a) + \hat p_k(s,a)^\top \bar V_k + b_k(s,a).
\end{align*}
We assume that $b_k^{rw}(s,a) \sim \sqrt{\frac{\log(M(1\lor n_k(s,a)))/\delta}{(1\lor n_k(s,a))}}$, where $M = \theta(n)$ and $b_k(s,a) \sim \sqrt{S}f_k(s,a)b_k^{rw}(s,a)$, where $f_k$ is a decreasing function in the number of visits to $(s,a)$ given by $n_k(s,a)$. One can verify that this is true for the the Q and value functions of StrongEuler.
\paragraph{Lower bound.}
We first show that for any $k$ it holds that $s_{2,1}$ is visited at least a constant fraction of $k$ times. Next, in a similar way we claim that $s_{5,i}, i>1$ are also visited a constant fraction of times. Finally this allows us to argue that for $\Omega(K)$ times the optimistic algorithm will try to solve the MDP problem starting from state $s_{2,1}$. Combining the fact that for this sub-MDP any state $s_{5,i},i>1$ is sub-optimal and the information theoretic lower bound for deterministic MDPs we see that the incurred regret would be at least $\Omega(n\log(K)/\epsilon)$.

\begin{lemma}
\label{lem:const_pulls}
It holds that $n_k(s_{2,1}) \geq \Omega(K)$ with probability at least $1-O(\delta\log(K))$. 
\end{lemma}
\begin{proof}
We first show that there exists constants $c,c'$ such that for all $k$ large enough it holds that $c n_k(s_{5,i}) \geq n_k(s_{5,j}) \geq c' n_k(s_{5,i})$ with high probability for $i,j>1$. Fix a $t>3$ and suppose that $s_{5,i}$ has been visited $t$ times. Let $\pi_{s_{5,i}}$ be the policy with highest optimistic value function after the $t$ times $s_{5,i}$ is visited. Suppose that there exists some $j$ which is only played $\gamma t$ times for some $\gamma < 1$ to be determined later. We can now consider the policy $\pi_{s_{5,j}}$ which follows $\pi_{s_{5,i}}$ up to layer $4$ and then chooses the action which transitions to state $s_{5,j}$. The probability that after $t$ plays of $\pi_{s_{5,i}}$, $\pi_{s_{5,i}}$ is played again before $\pi_{s_{5,j}}$ is bounded by
\begin{align*}
    &\PP\left(\hat r_{s_{5,i}}(t) + 2\sqrt{\frac{\log(Mt/\delta)}{t}} \geq \hat r_{s_{5,j}}(\gamma t) + 2\sqrt{\frac{\log(\gamma Mt/\delta)}{\gamma t}}\right)\\
    &\leq \PP\left(\hat r_{s_{5,i}}(t) - \sqrt{\frac{\log(Mt/\delta)}{t}} \geq \hat r_{s_{5,j}}(\gamma t) + \sqrt{\frac{\log(\gamma Mt/\delta)}{\gamma t}}\right)\\
    &\leq \PP\left(\hat r_{s_{5,i}}(t) - \sqrt{\frac{\log(Mt/\delta)}{t}} \geq 1/10\right) + \PP\left(\hat r_{s_{5,j}}(\gamma t) + \sqrt{\frac{\log(\gamma Mt/\delta)}{\gamma t}} \leq 1/10\right) \leq \frac{2\delta}{M\gamma t},
\end{align*}
\cd{Should $\hat r_{s_{5,i}}$ be $\hat r_{s_{5,j}}$ on the RHS?} 
where we have chosen $\gamma$ sufficiently small (e.g. 0.001) so that $3\sqrt{\frac{\log(Mt/\delta)}{t}} \leq \sqrt{\frac{\log(\gamma Mt/\delta)}{\gamma t}}$ \cd{Should this be $3\sqrt{\frac{\log(Mt/\delta)}{t}} \leq \sqrt{\frac{\log(\gamma Mt/\delta)}{\gamma t}}$?} . Now if we assume that there exists a $k$ during which $c n_k(s_{5,i}) \geq n_k(s_{5,j})$ for sufficiently small $c$ this implies that there exists a $t$ at which $\hat r_{s_{5,i}}(t) + 2\sqrt{\frac{\log(Mt/\delta)}{t}} \geq \hat r_{s_{5,j}}(\gamma t) + 2\sqrt{\frac{\log(\gamma Mt/\delta)}{\gamma t}}$ and so $c n_k(s_{5,i}) < n_k(s_{5,j})$ with probability $1- O(\log(K)\delta)$. The other direction of the inequality follows in a similar way. For the rest of the proof we can now assume that at any $k$ the number of times two policies visiting $s_{2,2}$ have been played differs by at most a constant, otherwise this would be a contradiction with $c n_k(s_{5,i}) \geq n_k(s_{5,j}) \geq c' n_k(s_{5,i})$ for $i>1$. Further, in a similar way we can show the same result for all optimal policies which visit $s_{2,1}$.

Fix $tn \in [K]$ and $\gamma > 1$ to be determined later. Suppose that $s_{2,1}$ has been visited $tn$ times and $s_{2,2}$ has been visited $\gamma tn$ times. We now compute the probability that $s_{2,2}$ is visited before $s_{2,1}$. Let $\pi^*_{1}$ be the optimal policy visiting $s_{2,1}$, which has been played most often out of all optimal policies visiting $s_{2,1}$. Under our assumption we know that $\pi^*_{1}$ has been visited at most $c_1 t$ times for some constant $c_1$. Let $\pi^*_2$ be the optimal policy visiting $s_{2,2}$ which has been visited least often among all policies visiting $s_{2,2}$. Again, under our assumption $\pi^*_2$ has been played at most $c_2 \gamma t$ times.
Denote by $\hat V^{\pi^*_{1}}(t)$ the optimistic value function after visiting $s_{2,1}$, $t$ times. Because the rewards and transitions are deterministic for $\pi^*_{1}$, except on $s_{4,1}$, it holds that $\hat V^{\pi^*_{1}}(c_1 t) \geq 1/2 + \epsilon + b_{\pi^*_1}(c_1 t) - \sqrt{\frac{\log(Mc_1 t/\delta)}{c_1 t}}$ with probability $1-\delta$ over all rounds. Here $b_{\pi^*_{1}}(c_1 t)$ is the sum of all the bonuses for states visited by $\pi^*_{1}$ after $c_1 t$ rounds in which $s_{2,1}$ has been visited and $a$ is the action at $s_{4,1}$ which transitions to $s_{5,1}$.
Our choice of $\pi^*_2$ implies
\begin{align*}
    \hat V^{\pi^*_2}(c_2 \gamma t) \leq 3/12 + \epsilon + \hat r_{s_{4,1},\pi^*_2}(c_2\gamma t)+ \hat r_{s_{5,i},\pi^*_2}(c_2\gamma t) + b_{\pi^*_2}(c_2\gamma tn),
\end{align*}
where $\hat r_{s,\pi}(c_2 t)$ is the empirical mean of the reward for state-action pair $(s,\pi(s))$ after visiting the state-action pair $c_2 t$ times.
We now compute the probability that $s_{2,2}$ is visited before $s_{2,1}$ is visited $n$ times. This probability is bounded by the probability to play $\pi^*_2$ before $\pi^*_1$
\begin{align*}
    &\PP(\hat V^{\pi^*_1}(c_1 t) \leq \hat V^{\pi^*_2}(c_2\gamma t)) \leq\\
    &\PP\left(1/2 + \epsilon + b_{\pi^*_1}(c_1 t) - \sqrt{\frac{\log(Mc_1 t/\delta)}{c_1 t}} \leq  3/12 + \epsilon + \hat r_{s_{4,1},\pi^*_2}(c_2 \gamma t)+ \hat r_{s_{5,i},\pi^*_2}(c_2 \gamma t) + b_{\pi^*_2}(c_2 \gamma t)\right).
\end{align*}
Choose $\gamma$ so that the bonuses satisfy 
\begin{align*}
    \sqrt{\frac{\log(c_1Mt/\delta)}{c_1t}} \geq 3\sqrt{\frac{\log(c_2\gamma Mt/\delta)}{c_2\gamma t}}.
\end{align*}
This implies 
\begin{align*}
    &\PP(\hat V^{\pi^*_1}(c_1 t) \leq \hat V^{\pi^*_2}(c_2 t))\\
    &\leq \PP\left(1/6 \leq \hat r_{s_{4,1},\pi^*_2}(c_2\gamma t)+ \hat r_{s_{5,i},\pi^*_2}(c_2\gamma t) - 4\sqrt{\frac{\log(c_2\gamma Mt/\delta)}{c_2\gamma t}}\right) \leq \frac{\delta}{c_2\gamma tM},
\end{align*}
where the first inequality follows by just considering the difference of bonuses for the rewards at each state-action pair visited by $\pi^*_1$ and $\pi^*_2$ and our choice of $\gamma$ and the second inequality follows because $\hat r_{s_{4,1},\pi^*_2}(c_2\gamma t)+ \hat r_{s_{5,i},\pi^*_2}(c_2\gamma t)$ is a sum of $2\gamma t$ independent Bernoulli variables. The above implies that $s_{2,1}$ is selected at least $n$ times before $s_{2,2}$ with probability $1-O(\delta\log(K))$. In particular for every $O(n)$ iterations of the optimistic algorithm we must have that $s_{2,1}$ is visited at least $O(n)$ times, otherwise there exists a $t$ for which $\hat V^{\pi^*_1}(c_1 t) \leq \hat V^{\pi^*_2}(c_2\gamma t)$.
\end{proof}

We can now show the lower bound.
\begin{theorem}
\label{thm:lower_bound_det_opt}
There exists an MDP instance with deterministic transitions on which any optimistic algorithm with $\delta \leq O(1/\log(K))$ will incur expected regret at least $\Omega(S\log(K)/\epsilon)$ while it is information theoretically possible to achieve $O(\log(K)/\epsilon)$ regret.
\end{theorem}
\begin{proof}
Lemma~\ref{lem:const_pulls} implies that with constant probability the optimistic algorithm will visit $s_{2,1}$ in the MDP in Figure~\ref{fig:mdp_det_lower} at least $\Omega(K)$. For the rest of the proof condition on this event. Because optimistic algorithms disregard all states which can not be visited from $s_{2,1}$ once they are in $s_{2,1}$ we can restrict our attention on the sub-MDP with starting state $s_{2,1}$. Further Lemma~\ref{lem:const_pulls} implies that the total number of times we have played a policy visiting $s_{2,2}$ as opposed to one visiting $s_{2,1}$ is at most a multiplicative constant $c$ more. This, together with the proof of Theorem~\ref{thm:lower_bound_gen} implies that the expected regret of any uniformly good algorithm on the sub-MDP is governed by the following LP
\begin{align*}
    \minimize{\alpha(\pi)\geq 0,\eta(\pi)\geq 0}{\sum_{\pi \in \Pi} \eta(\pi)\left(\return{*}_{\theta} - \return{\pi}_{\theta}\right)}
    {
    \sum_{\pi \in \Pi} \alpha(\pi) KL(\PP_\theta^\pi,\PP_\lambda^\pi) \geq 1 \qquad \textrm{for all } \,\,\lambda \in \Lambda(\theta)\\
    &&&\sum_{\pi\in\Pi} \alpha(\pi) \leq c\sum_{\pi\in \Pi}\eta(\pi)
    },
\end{align*}
i.e., we can assume that every policy is played roughly $c\eta(\pi)$ times instead of $\eta(\pi)$ times. Now following the proof of Theorem~\ref{thm:lower_bound_deterministic}, we can reduce the above problem to finding a feasible solution for the dual LP on the restricted set of confusing environments $\breve \Lambda(\theta)$ which only changes the rewards at states $s_{5,i},i>1$ or $s_{4,2}$. This dual LP is
\begin{align*}
    \maximize{\mu(\lambda)\geq 0,\mu_\alpha\geq 0}{\sum_{\lambda \in \breve \Lambda(\theta)} \mu(\lambda)}
    {
    c\mu_\alpha \leq v^*_\theta - v^{\pi}\qquad \textrm{for all } \,\,\pi \in \Pi\\
    &&&\sum_{\lambda \in \breve\Lambda(\theta)}\mu(\lambda)KL(\PP^{\pi}_\theta, \PP^{\pi}_\lambda) \leq \mu_\alpha\qquad \textrm{for all } \,\,\pi \in \Pi
    }.
\end{align*}
Arguing in the same way about feasibility as in Theorem~\ref{thm:lower_bound_deterministic} shows that the expected regret of any uniformly good strategy on the sub-MDP for large enough $K$ is lower bounded by $\Omega(n\log(K)/\epsilon)$. This implies the claim of the theorem and completes the proof.
\end{proof}
